# Supplementary material for: An Information Theoretic Perspective on Conformal Prediction
Source: arXiv:2405.02140 source file (2025-02-14)
Supplement: Supplementary file 1 [file algo.tex]

\SetInd{0.75em}{0.5em}
\DontPrintSemicolon
\SetKwComment{Comment}{// }{}
\begin{algorithm}[H]
\caption{Conformal training algorithm.} \label{alg:conftr}
\SetKwInOut{Input}{input}
\SetKwInOut{Output}{output}
\Input{A batch of labeled samples $\gB$, a model $f$, a loss function $\gL$ that can be any of our upper bounds (\ref{eq:dpi_bound}), (\ref{eq:mb_fano_bound}) or (\ref{prop:simple_fano}) or a version of (\ref{eq:size_loss})---see variants (\ref{eq:bel_loss}) and (\ref{eq:cftr_class}) in Appendix~\ref{app:conftr}.}
\For{\upshape{each training batch} $\gB$}{ 
    split $\gB$ into $\gB_{cal}$ and $\gB_{test}$\;
    \For{\upshape{each} $(x_i, y_i) \in \gB_{cal}$}{
        compute score $s_i = s_f(x_i, y_i)$\;
    }
    sort scores (in a differentiable manner) obtaining $s_{(1)} < s_{(2)} < \ldots < s_{(|\gB_{cal}|)}$\;
    set $\hat q = s_{(\lceil(|\gB_{cal}|+1)(1-\alpha)\rceil)}$  \Comment*[r]{get $1-\alpha$ quantile estimate using $\gB_{cal}$}
    \For{\upshape{each} $(x_j, y_j) \in \gB_{test}$}{
        \For{\upshape{each} $y \in \gY$}{
            $\hat \gC_f(x_j, y) \gets \sigma(\hat q - s_f(x_j, y))$ \Comment*[r]{Construct soft prediction set}
        }
    }
    \Comment*[l]{Bounds (\ref{eq:dpi_bound}) and (\ref{eq:mb_fano_bound}) also require class probabilities under $Q$, which in this case are given by the model $f(x_j)$}
    compute loss according to $\gL$ on $\gB_{test}$ using $y_j, \hat \gC_f(x_j)$ and if needed $f(x_j)$ \;
    update $f$ via gradient descent to minimize loss
}
\end{algorithm}
